# Supplementary material for: Mirror Sinkhorn: Fast Online Optimization on Transport Polytopes
Source: arXiv:2211.10420 source file (2023-06-20)
Supplement: Supplementary file 1 [file supplements.tex]

\documentclass[twoside]{article}

\usepackage{aistats2023}
% If accepted, instead use the following line for the camera-ready submission:
% \usepackage[accepted]{icml2023}

% For theorems and such
\usepackage{amsmath}
\usepackage{amssymb}
\usepackage{mathtools}
\usepackage{amsthm}

% if you use cleveref..
\usepackage[capitalize,noabbrev]{cleveref}

%%%%%%%%%%%%%%%%%%%%%%%%%%%%%%%%
% THEOREMS
%%%%%%%%%%%%%%%%%%%%%%%%%%%%%%%%
\theoremstyle{plain}

\theoremstyle{definition}

\theoremstyle{remark}

%%%%%%%%%%%%%%%% Commandes %%%%%%%%%%%%%%%%

% Recommended, but optional, packages for figures and better typesetting:
\usepackage{xcolor}
\usepackage{microtype}
\usepackage{graphicx}
\usepackage{subfigure}
\usepackage{booktabs}
% for professional tables
\usepackage[algo2e]{algorithm2e} 
\usepackage{float}
\usepackage{amsfonts}
\usepackage{graphicx}
\usepackage{bbm}
\usepackage{float}
\usepackage[colorlinks=true,citecolor=blue,allcolors=blue]{hyperref}
\usepackage{etoolbox}
\usepackage{breakcites}

\begin{document}
\onecolumn
\aistatstitle{Mirror Sinkhorn://
Supplementary Materials}

\input{sections/5-appendix}
\bibliographystyle{plain}
\bibliography{references}
\end{document}
